# Supplementary material for: InterHandGen: Two-Hand Interaction Generation via Cascaded Reverse Diffusion
Source: arXiv:2403.17422 source file (2024-03-26)
Supplement: Supplementary file 1 [file supp_diversity.tex]

\begin{table}[!h]
\centering
{ \small
\setlength{\tabcolsep}{0.2em}

\caption{\textbf{.}} 
\label{table:supp_diversity}
\vspace{-0.5\baselineskip}
\begin{tabularx}{\columnwidth}{>{\centering}m{3cm}|Y|Y}
\toprule
Method & Ours & Ours w/ Aug. \\
\midrule 
Diversity $\uparrow$ & 3.59 & \textbf{4.39} \\
\bottomrule
\end{tabularx}}
\end{table}
