# Supplementary material for: InterHandGen: Two-Hand Interaction Generation via Cascaded Reverse Diffusion
Source: arXiv:2403.17422 source file (2024-03-26)
Supplement: Supplementary file 2 [file supp_layer_conf.tex]

\begin{table*}[h]
\centering
{ \small
\setlength{\tabcolsep}{0.2em}

\caption{Layer configurations of our diffusion model $D_{\theta}$.}
\vspace{-0.5\baselineskip}
\label{table:layer_configuration}

\begin{tabularx}{\textwidth}{>{\centering}m{2.6cm}|>{\centering}m{8.4cm}|Y}
\toprule
 & Layer Description & Output Dimension \\
\midrule
TCNN-1 & (Temporal conv., filter size 3, 96 features, stride 2) & $J \times 96 \times 8$ \\
TCNN-2 & (Temporal conv., filter size 3, 64 features, stride 2) & $J \times 64 \times 3$ \\
TCNN-3 & (Temporal conv., filter size 3, 64 features, stride 1) & $J \times 64 \times 1$ \\
\midrule
MLP-1 & (Linear, 128 features) & $J \times 128$ \\
MLP-2 & (Linear, 64 features) & $J \times 64$ \\
MLP-3 & (Linear, 14 ($= 6N+3$) features) & $J \times 14 \, (= 6N+3)$ \\
\bottomrule
\end{tabularx}
}
\end{table*}
